# Supplementary material for: Health Text Simplification: An Annotated Corpus for Digestive Cancer Education and Novel Strategies for Reinforcement Learning
Source: arXiv:2401.15043 source file (2024-11-10)
Supplement: Supplementary file 1 [file response_document1.tex]

\documentclass[review, sort&compress]{elsarticle}

%\usepackage[letterpaper, portrait,  rmargin=2.0in]{geometry}
\usepackage[letterpaper, portrait, margin=1.0in]{geometry}
\usepackage{booktabs}

\usepackage[color=yellow,textwidth=1.5in,textsize=small]{todonotes}
\usepackage{xcolor}
\usepackage{hyperref}
\usepackage{soul}
%http://latexcolor.com/
\definecolor{comment_color}{rgb}{0.0, 0.18, 0.65}
\definecolor{internal_color}{rgb}{0.79, 0.0, 0.09}


\bibliographystyle{bst/vancouver}
\AtBeginDocument{\colorlet{default_color}{.}}

\usepackage{parskip}

%\color{comment_color}
%\color{default_color}  


\begin{document}

\noindent
{\huge Reviewer Response Document \par}
\bigskip

We carefully read the reviewer comments and have edited the manuscript to address as many points as possible. We interleaved our responses with the reviewers’ comments below, to provide context for the responses. A version of the manuscript indicating the associated changes is provided with the revised manuscript.

\section*{Associate Editor’s comments}

Both reviewers raised some major concerns, such as data license issues, limited data size, and missing relevant work. Please carefully address all comments from both reviewers and submit a revised manuscript.

\color{comment_color}

\textbf{RESPONSE:} We appreciate the feedback from the Associate Editor and reviewers. We have carefully addressed each point raised and extensively revised the manuscript, including substantial new experimentation. \\

\color{default_color} 

\section*{Reviewer: 1}

This paper introduces the Simplified Digestive Cancer (SimpleDC) corpus. This corpus consists of parallel cancer education materials from the American Cancer Society, Centers for Disease Control and Prevention, and National Cancer Institute. The study explores various large language model (LLM)-based simplification methods, including fine-tuning, reinforcement learning (RL), and reinforcement learning with human feedback (RLHF). The paper highlights the efficacy of a novel RLHF reward function in enhancing model performance on unlabeled data and demonstrates that RL/RLHF methodologies can effectively adapt out-of-domain text simplification models to targeted domains.

Strengths:

1. Innovative Corpus: The introduction of the SimpleDC corpus, specifically tailored for digestive cancer education, addresses a significant gap in health text simplification resources.

2. Advanced Methodologies: The study employs state-of-the-art LLMs and explores a wide range of learning approaches, including a novel RLHF reward function that outperforms existing methods.


Weaknesses:

1. License Issues and Dataset Comparison: The paper does not discuss the license issues related to using and releasing data from sources like the National Cancer Institute (NCI), the American Cancer Society (ACS), and the Centers for Disease Control (CDC). 

\color{comment_color}
\textbf{RESPONSE:} We acknowledge the concern regarding license issues related to using data from the NCI, ACS, and CDC. Although obtaining explicit permission from these organizations may be challenging, we believe our use of this data aligns with fair use principles. These sources are well-attributed in the paper, and the text is used solely for academic research purposes to advance NLP and public health informatics. Our use of the data is consistent with its intended purpose, namely the dissemination of critical health information, and we used the minimal amount of text necessary to advance our research. Importantly, our use does not substitute for or diminish the value of the original content; instead, it presents approaches for improving it. We hope these points adequately address the reviewer’s comment. The release of the annotated corpus will include detailed attribution of the sources, such that each sample can be traced to the original source webpage. \\

\color{default_color} 

Additionally, a comparison and discussion of the differences and advantages between the proposed dataset and existing text simplification datasets would enhance the study's comprehensiveness.

\color{comment_color}
\textbf{RESPONSE:} We update the introduction and related work sections to better articulated how our dataset, SimpleDC, is different from other health simplification datasets. \\

\color{default_color} 

2. Limited Data Size: The limited size of the SimpleDC dataset raises concerns about its sufficiency for training efficient models. Larger datasets would provide more robust training data and potentially improve model performance.

\color{comment_color}

\textbf{RESPONSE:} Thank you for your feedback regarding the size of the SimpleDC train dataset. We acknowledge that the train set is relatively small and that a larger training set would likely improve model performance. However, creating such a dataset, especially one annotated by subject matter experts, is both costly and labor-intensive. The SimpleDC dataset represents a significant effort to provide high-quality, annotated data for the specific domain of digestive cancer education, and expanding it would require substantial resources. Our study explores leveraging pretrained LLMs to achieve high performance in low-resource settings, and the results demonstrate high performance can be achieved even with limited data. We believe this work is an important step towards developing robust models for specialized applications where large annotated datasets are not readily available. We have updated the results section to highlight this.\\

\color{default_color} 

3. Missing Relevant Studies: The paper overlooks many relevant studies[1][2][3][4], particularly recent progress on LLMs for text simplification. Including these studies would provide a more comprehensive overview of the current state of the field.

\color{comment_color}

\textbf{RESPONSE:} We appreciate the reviewer’s suggestion to include additional related studies. We have carefully reviewed the suggested references and included them in our manuscript to provide a more comprehensive overview of recent advancements in LLMs for text simplification. \\


\color{default_color} 

4. Reorganization of Related Work Section: The related work section should be reorganized into sub-sections to better summarize related studies on text simplification methods, text simplification datasets, and SFT/RLHF in LLMs.

\color{comment_color}

\textbf{RESPONSE:} We have reorganized the Related Work section as suggested. The updated version is now subdivided into four subsections: text simplification task, health text simplification, general domain text simplification, and simplification with reinforcement learning.\\


\color{default_color} 

5. Comparison with More LLMs: The comparison in Table 2 should include more LLMs, such as LLaMA2 13B, LLaMA2 70B, gemini, and LLaMA3 models, to provide a more comprehensive comparison of model performance.

\color{comment_color}

\textbf{RESPONSE:} We have expanded our experimentation to include Meta's LLaMA 3 variants, specifically the 8 billion and 70 billion parameter versions (LLaMA-3-8B and LLaMA-3-70B). These additions provide a more comprehensive comparison of model performance, addressing the breadth and size of models. We did not include Gemini or larger versions of LLaMA 2 (such as LLaMA-2-13B or LLaMA-2-70B) because LLaMA 3 reportedly outperforms these models in many tasks\footnote{\url{https://ai.meta.com/blog/meta-llama-3/}}. Table 2 presents the updated results, including the addition of these models. We extensively edited the manuscript, including the introduction, results, discussion, and conclusions, to address the addition of these models. These additional LLMs enhance the robustness and comprehensiveness of our comparative analysis.\\


\color{default_color} 

Overall, while the paper makes significant contributions to health text simplification, addressing these weaknesses would strengthen its impact and comprehensiveness.

[1] Feng, Y., Qiang, J., Li, Y., Yuan, Y., \& Zhu, Y. (2023). Sentence simplification via large language models. arXiv preprint arXiv:2302.11957.

[2] Lu, Junru, et al. "NapSS: paragraph-level medical text simplification via narrative prompting and sentence-matching summarization." Findings of the Association for Computational Linguistics: EACL 2023 (2023): 1079-1091. APA

[3] Luo, Z., Xie, Q., \& Ananiadou, S. (2022, December). Readability Controllable Biomedical Document Summarization. In Findings of the Association for Computational Linguistics: EMNLP 2022 (pp. 4667-4680).

[4] Ryan, Michael J., Tarek Naous, and Wei Xu. "Revisiting non-English text simplification: A unified multilingual benchmark." arXiv preprint arXiv:2305.15678 (2023).

\section*{Reviewer 2}

This paper tackles the health text simplification task with large language models. For this, the authors curated a corpus SimpleDC of ~1k sentence pairs for digestive cancer patient education. Based on SimpleDC and the existing Med-EASi corpora, the authors conducted many experiments, including SFT \& RLHF of open LLMs, and prompting close LLMs. While the RLHF is naively done, this is still one of the first studies I see in medicine conducting RLHF. The evaluations include automatic metrics, pair-wise comparison conducted manually, as well as error analysis. The proposed model achieved good performance. Overall, this is an interesting paper for an important task. The presentations are mostly clear and the article is easy to follow. My concerns are listed below:

Major:
1. Model sizes. It seems that authors have only fine-tuned 7B llama 2. Any reasons not doing larger models (e.g., the 70B version)? In addition, the authors might also want to add the GPT-3.5-Turbo results.

\color{comment_color}

\textbf{RESPONSE:} In response to your feedback and the feedback from Reviewer 1, we expanded the experimentation to include Llama-3-8B and Llama-3-70B. The manuscript, including the results in Table 2, reflects these additional experiments. We did not include larger versions of Llama 2 (such as Llama-2-13B or Llama-2-70B) because Llama 3 has been reported to outperform these models in most tasks\footnote{\url{https://ai.meta.com/blog/meta-llama-3/}}. We also did not include GPT-3.5-Turbo results because GPT-4 reportedly outperforms GPT-3.5 in most of the tasks\footnote{\url{https://openai.com/index/gpt-4-research/}}.\\

\color{default_color} 

2. RLHF. It seems different from the original InstructGPT where the reward model is explicitly trained with human preferences. Here the reward model uses an original/simple classifier + direct optimization of the readability metric. The authors might want to provide more discussions on the discrepancy and why they didn't use the original version.

\color{comment_color}

\textbf{RESPONSE:} We have taken inspiration from the InstructGPT \cite{NEURIPS2022_b1efde53} framework and other state-of-the-art techniques such as TESLEA \cite{phatak2022medical}. Our OvS (Original vs. Simplified) reward model functions similarly to the reward model used in InstructGPT, where human preferences play a critical role. Specifically, we use a classifier trained to distinguish between original and simplified texts, leveraging the SimpleDC dataset's annotations to incorporate human-like judgment into the model. This classifier provides a probabilistic reward signal that aligns with human preferences for simplified text.

We have expanded our discussion in the manuscript (Section 3.2.2 in Original vs. Simplified (OvS) Reward) to clarify this and to highlight how our reward model aligns with the original InstructGPT framework. Our approach also incorporates the FKGL readability metric to enhance the model's focus on text simplicity, similar to the TESLEA approach. Our methodology aims to balance fidelity to the original text and readability, aligning closely with human judgment. This approach ensures our model simplifies text effectively while maintaining its core meaning. In Table 2, we present the performance with and without the addition of the FKGL reward \textit{(Exp. No. 08 vs 09 and Exp. No. 12 vs 13)} to illustrate the impact of this reward.\\

\color{default_color} 

3. The authors report that GPT-4 alter the meaning of the original sentences by a lot in the simplification. Is it possible a better prompting strategy can solve this? The authors might want to explore this approach.

\color{comment_color}

\textbf{RESPONSE:}  Thank you for your comment regarding the potential for improved prompting strategies. We conducted extensive prompt engineering to optimize the performance of our models, including the presented prompting strategies.  While additional prompt engineering may mitigate some issues, our primary focus in this paper has been on refining the RLHF approach to improve the overall quality of text simplification. \\

\color{default_color} 

4. Do you have the inter-annotator agreement data for the preference evaluations? With such human annotations, would it be possible to study how a LLM judge (e.g., GPT-4) correlate with human judgements? If so, one can simply use the GPT-4 judge to scale the evaluations.

\color{comment_color}

\textbf{RESPONSE:} To ensure annotation quality, we double-annotated the development and test sets and had a third annotator review these annotations to determine their preference. The third annotator almost always deemed one or both of the annotations to be of high quality, indicating consistent annotation standards. However, the third annotator did not exhibit a strong preference for the annotations of any single annotator. Traditional inter-annotator agreement metrics, such as Cohen's Kappa, are not well-suited for this task.

The use of LLMs as evaluators is a compelling and growing area of research. Employing GPT-4 or another LLM as an evaluator for this text simplification project is an intriguing possibility. However, as the reviewer points out, it is essential to study and validate the correlation between LLM judgments and human judgments before adopting this approach. This line of inquiry could be incorporated into future research on reinforcement learning from AI feedback.\\

\color{default_color} 

5. Please have a case study table showing the simplification outputs of the same sentence(s) by different models.

\color{comment_color}

\textbf{RESPONSE:} We have added a table in the appendix (Appendix A. Case Study of Simplification Outputs) that illustrates the outputs generated by various models for the same original sentence. This table provides a clear comparison of the simplifications produced by different models, highlighting their respective approaches to text simplification.\\


\color{default_color} 

6. Relevant reviews should be cited, e.g.: https://academic.oup.com/bib/article/25/1/bbad493/7505071.

\color{comment_color}

\textbf{RESPONSE:} We have reviewed and included the suggested paper, as well as additional papers, to improve the completeness of the related work section.\\

\color{default_color} 

Minor:

The size of SimpleDC should be clearly mentioned in the abstract. A table might be needed to summarize the key statistics of the SimpleDC corpus (size, length, etc).

\color{comment_color}

\textbf{RESPONSE:} As suggested, we added the corpus size to the abstract and an additional table \textit{(Table 1)} presenting some key statistics of the SimpleDC corpus.\\

\color{default_color} 

Page 7 Line 20: ``encoder-only LLMs'' should be ``decoder-only LLMs'', I hope this is a typo instead of a misunderstanding.

\color{comment_color}
\textbf{RESPONSE:} Yes, this was a typo. We have corrected the error on section 3.2, changing ``encoder-only LLMs'' to ``decoder-only LLMs.'' \\

\color{default_color} 

The authors might need to explain how each metric is calculated, especially SARI which is not very common.

\color{comment_color}
\textbf{RESPONSE:} We have updated the Evaluation section (section 3.3) to include detailed explanations of each metric with particular emphasis on SARI. SARI evaluates text simplification quality by measuring additions, deletions, and substitutions, reflecting the system's effectiveness in modifying the input text while preserving its original meaning.\\

\color{default_color} 

In each table, the authors might also need to label for each score whether higher is better (e.g., for FKGL, it is the lower the better, right?)

\color{comment_color}
\textbf{RESPONSE:} We have updated the tables to indicate the desired direction for each metric. Specifically, we annotated the tables to show that higher scores are better for SARI, BLEU, BERTScore, and ROUGE ($\uparrow$), while lower scores are better for FKGL ($\downarrow$). This provides clearer guidance on interpreting these metrics. Please see the revised Table 2 in the updated manuscript, which includes these annotations for improved clarity.\\

\color{default_color} 

\bibliography{mybib}
%\bibliographystyle{acl_natbib}




\end{document}
