# Supplementary material for: Health Text Simplification: An Annotated Corpus for Digestive Cancer Education and Novel Strategies for Reinforcement Learning
Source: arXiv:2401.15043 source file (2024-11-10)
Supplement: Supplementary file 2 [file response_document2.tex]

\documentclass[review, sort&compress]{elsarticle}

%\usepackage[letterpaper, portrait,  rmargin=2.0in]{geometry}
\usepackage[letterpaper, portrait, margin=1.0in]{geometry}
\usepackage{booktabs}

\usepackage[color=yellow,textwidth=1.5in,textsize=small]{todonotes}
\usepackage{xcolor}
\usepackage{hyperref}
\usepackage{soul}
%http://latexcolor.com/
\definecolor{comment_color}{rgb}{0.0, 0.18, 0.65}
\definecolor{internal_color}{rgb}{0.79, 0.0, 0.09}


\bibliographystyle{bst/vancouver}
\AtBeginDocument{\colorlet{default_color}{.}}

\usepackage{parskip}
\usepackage{framed}

%\color{comment_color}
%\color{default_color}  


\begin{document}

\noindent
{\huge Reviewer Response Document \par}
\bigskip

We carefully read the reviewers' comments and have edited the manuscript to address the minor suggestions made by the reviewers. We interleaved our responses with the reviewers’ comments below, to provide context for the responses. A version of the manuscript indicating the associated changes is provided with the revised manuscript.

\section*{Associate Editor’s comments}

Please address additional minor comments and submit a revised manuscript.

\color{comment_color}

\textbf{RESPONSE:} We have updated our manuscript to address all reviewer feedback. \\

\color{default_color} 

\section*{Reviewer: 1}

I appreciate the authors' effort in addressing most of the concerns raised in the initial review. The revisions have improved the manuscript. However, there are a few issues that I would suggest addressing before the manuscript is ready for publication:

1) Graphical Abstract: The figure currently used for the graphical abstract needs to be replaced with a high-resolution version.

\color{comment_color}
\textbf{RESPONSE:} We have updated the graphical abstract to a high-resolution version. \\

\color{default_color} 

2) Legal Usage of Data Sources: it would benefit from an explicit discussion and illustration regarding the legal aspects of utilizing data from sources such as the National Cancer Institute (NCI), the American Cancer Society (ACS), and the Centers for Disease Control and Prevention (CDC).

\color{comment_color}


\textbf{RESPONSE:} We have added the following description to Section 7: Data Availability and Legal Considerations of the manuscript:

\begin{quote}
    ``We provide the new SimpleDC corpus to the research community to advance health text simplification.\footnote{\href{https://github.com/mushfiqur11/simpledc-dataset.git}{https://github.com/mushfiqur11/simpledc-dataset.git}} In developing SimpleDC, we utilized publicly available text data from the NCI, ACS, and CDC websites with the goal of advancing text simplification and public health communication. Our use of this data is in alignment with fair use principles, as the data was employed exclusively for academic and research purposes, without any commercial intent. We minimized data usage, extracting only the portions necessary to support our work on text simplification and public health communication. Furthermore, our use of the data does not adversely affect the market value or potential of the original content. The text data from the NCI, ACS, and CDC was specifically used to improve NLP methods that enhance the accessibility of health information, with all sources carefully attributed. SimpleDC is made publicly available, with detailed source attribution, ensuring full transparency and traceability."
\end{quote}
\color{default_color} 

3) Enhancing the Data Annotation Section: Given that one of the main contributions of the paper is the introduction of a new annotated dataset, I recommend that the authors provide additional details about the data annotation process. Such as, the details of annotation guidelines, details of annotation experts. To further substantiate the quality of the annotations, I suggest including statistical metrics such as the Inter-Annotator Agreement (IAA) scores.

\color{comment_color}
\textbf{RESPONSE:}  We appreciate the reviewer’s suggestion to further enhance the data annotation section. We have included additional details about the annotation process and the expertise of the annotators. Regarding IAA, we added the following justification for the annotator agreement approach:

\begin{quote}
    ``Since text simplification is a generative task without categorical labels, traditional inter-annotator agreement (IAA) metrics, like Cohen’s Kappa, are not well suited. Instead, we evaluated annotation quality by having two annotators create the simplified text and then having a third annotator assess their preference for simplifications.''
    \end{quote}


\color{default_color} 

\section*{Reviewer: 2}
Thank you for addressing my concerns. There are still typos like "GPT4" (should be "GPT-4") in the manuscript. Please carefully proofread and fix them.

\color{comment_color}
\textbf{RESPONSE:} 
Thank you for the reviews. We have fixed these typos.

\color{default_color} 


\end{document}
